# Supplementary material for: Task Singular Vectors: Reducing Task Interference in Model Merging
Source: arXiv:2412.00081 source file (2025-04-04)
Supplement: Supplementary file 1 [file appendix.tex]

% % da qui in poi è il paper è stato usato come una lavagna


% \[
% S_u = \left[
% \begin{array}{c|c}
%    1 & \langle u^1, u^2 \rangle^2 \\
% \hline
%    \langle u^2, u^1 \rangle^2 & 1
% \end{array}
% \right]
% \]


% Normalizing  by rows we obtain 
% $$ W_{u} = \left [
%  \begin{array}{c|c}
%   \frac{1}{ 1 + <u_{1}^1, u_1^2 >^2 } % qui gli indici vogliono dire primo vettore singolare e gli esponenti significano del primo o del secondo task (per gli u, gli esponenti dei sigma sono potenze)
%   & \frac{<u_{1}^1, u_1^2 >^2}{ 1 + <u_{1}^1, u_1^2 >^2} \\
%   \\
% \hline
% \\
%   \frac{<u_1^2, u_{1}^1>^2 }{ 1 + <u_1^2, u_{1}^1>^2 }&
%   \frac{1}{ 1 + <u_1^2, u_{1}^1>^2}
%  \end{array} 
% \right]  
% $$ % okay!


% \[
% S_v = \left[
% \begin{array}{c|c}
%    1 & \langle v^1, v^2 \rangle^2 \\
% \hline
%    \langle v^2, v^1 \rangle^2 & 1
% \end{array}
% \right]
% \]

% Normalizing dividing each element by the sum of its columns we obtain 

% $$ W_{v} = \left [
%  \begin{array}{c|c}
%   \frac{1}{ 1 + \langle v^2, v^1 \rangle^2 } 
%   & \frac{<v_{1}^1, v_1^2>^2}{1 + <v_{1}^1, v_1^2>^2} \\
%   \\
% \hline
% \\
%  \frac{<v_{1}^1, v_1^2>^2}{1 + \langle v^2, v^1 \rangle^2 }&
%    \frac{1}{1 + <v_{1}^1, v_1^2>^2 }
% \end{array}
% \right]  
% $$ 






% %$$ \Sigma (W_u \odot W_v) = \left [
% % \begin{array}{c|c}
% %  \frac{ \sigma_{1}^5}{ (\sigma_1^2 + \sigma_{2}^2 <u_{1}^1, u_1^2 >^2)(\sigma_1^2 + \sigma_{2}^2 <v_{1}^1, v_1^2>^2) } 
% %  & \frac{ \sigma_{1}^3 \sigma_2^2 <v_1^1, v_1^2>^2 <u_1^1,u_1^2>^2}{ (\sigma_1^2 +  \sigma_{2}^2 <u_{1}^1, u_1^2 >^2 )(\sigma_2^2 + \sigma_{1}^2  <v_{1}^1, v_1^2>^2)} \\
% %  \\
% %\hline
% %\\
% %\frac{  \sigma_{2}^3 \sigma_1^2 <v_{1}^1, v_1^2>^2  <u_{1}^1, u_1^2 >^2  }{ (\sigma_1^2 + \sigma_{2}^2  <v_{1}^1, v_1^2>^2 )(\sigma_2^2 +  \sigma_{1}^2 <u_{1}^1, u_1^2 >^2 ) }&
% %  \frac{ \sigma_{2}^5}{  (\sigma_2^2 +  \sigma_{1}^2 <u_{1}^1, u_1^2 >^2) (\sigma_2^2 +  \sigma_{1}^2  <v_{1}^1, v_1^2>^2 )}\\
% %\end{array}
% %\right]   $$ % okay 2!


% $$ (2W_u \odot \Sigma \odot 2W_v) = \left [
%  \begin{array}{c|c}
%   \frac{4 \sigma_1}{ (1 + <u_{1}^1, u_1^2 >^2)(1 + <v_{1}^2, v_1^1>^2) } 
%   & 0 \\
%   \\
% \hline
% \\
% 0 &
%   \frac{4 \sigma_{2}}{  (1 + <u_{1}^1, u_1^2 >^2) (1 + <v_{1}^1, v_1^2>^2 )}\\
% \end{array}
% \right]   $$

% Alternative writing:

% $$ (2W_u \odot \Sigma \odot 2W_v) = \left [
%  \begin{array}{c|c}
%   \frac{4 \sigma_{1}}{ (1 + \cos^2(\angle(u_{1}^1, u_1^2)))(1 + \cos^2(\angle(v_{1}^2, v_1^1))) } 
%   & 0 \\
%   \\
% \hline
% \\
% 0 &
%   \frac{4 \sigma_{2}}{  (1 + \cos^2(\angle(u_{1}^1, u_1^2)) (1 + \cos^2(\angle(v_{1}^1, v_1^2))}\\
% \end{array}
% \right]   $$


% $$ (2W_u \odot \Sigma \odot 2W_v) = \left [
%  \begin{array}{c|c}
%   \frac{4 \sigma_1}{ (\sum_{i=0}^k{<u_{1}^1, u_1^i>^2})(\sum_{j=0}^k{<v_{1}^j, v_1^1>^2}) } 
%   & 0 \\
%   \\
% \hline
% \\
% 0 &
%   \frac{4 \sigma_{2}}{ (\sum_{i=0}^k{<u_{1}^i, u_1^2>^2})(\sum_{j=0}^k{<v_{1}^j, v_1^2>^2})}\\
% \end{array}
% \right]   $$



% thoughts:
% \begin{enumerate}
%     \item each singular value is divided by a term where each singular value is affected by the inner product term that introduce an interaction between singular vectors.
%     \item the squared inner products means that the interaction of left and right singular vectors are weighted.
%     \item I suspect that the cosine term is an indication of the increase/decrease in volume of the contraction/expansion in each singular component, so this singular value normalization is performing a sort of reduction on the volume, to approximate the most prominent one, of the single transformation $\sigma_i u_i v_i^\top$. So if I look at each rank-one matrix as an independent transformation, where we have an interaction between tasks, we are modifying the rank-one by an interaction of more rank-one matrices, so more transformations means different volume and the indication of how much this difference is can be retrieved in the cosine term.
%     \item the similarity matrices tells us also that the rank of the merged task vector is not the sum of the rank of each compressed task since there is interaction between singular vectors, so could be $rank(\tau_{MT}) \leq rank(\sum_i \tau_i)$   

    
% \end{enumerate}
% what this matrix is doing:
% \begin{enumerate}
%     \item normalization of singular values by dividing for a term that involves the cosine similarity of singular vectors, this reduces/enhances the singular value depending on how close the directions of singular vectors are.
%     \item the singular vector inner product measures how aligned the singular vectors are, and then the squared term means that greater alignment (larger inner products) increases the denominator, and so reducing the transformed singular value (maybe this is a good point to expand on?) 
% \end{enumerate}


% $n $ numero di task 
% $k $ numero di singular vectors per task.

% $$ U [u_1^1 u_2^1 ...| u_1^2 u_2^2 ...| ...]$$


% $M = U \Sigma V^\top = \sum_{i=1}^n \sum_{j=1}^k \sigma_j^i u_j^i (v_{j}^i)^\top $


% $ \tilde{\Sigma} = W_u \odot \Sigma \odot W_v$


% \( \tilde{M} =  U \tilde{\Sigma}  V^\top = \sum_{i=1}^n \sum_{j}^k \tilde{\sigma}^i_{j} u_{j}^i (v_j^i)^\top \)

% If 

% $n = 2, k= 1$


% $M = \sigma_1 u_{1}^1 (v_{1}^1)^\top + \sigma_2 u_{1}^2 (v_{1}^2)^\top$ % somma di due matrici rank-1 con massimo dell'interferenza, tutta la seconda è ciò che non vorremmo e la prima è il desiderata (se ci fermassimo alla riga 5 dell' algoritmo per creare M)  

% Since $k = 1$ we can remove the subscript

% $M = \sigma_1 u^1 (v^1)^\top + \sigma_2 u^2 (v^2)^\top$ %same as before

% $ \tilde{M} = \tilde{\sigma}_{1} u^1 (v^1)^\top + \tilde{\sigma}_{2} u^2 (v^2)^\top . $ 

% Siamo nelle ipotesi 

% $v^1$ , $<v^1,v^2> >0$. 

% \begin{align*}
% M v^1 &= \sigma_1 u^1  + \sigma_2 < v^1, v^2> u^2 \\ % desiderata + unwanted (perchè v1 è del task 1) \\
%     \tilde{M} v^1 &= \tilde{\sigma}_{1} u^1 + \tilde{\sigma}_{2} <v^1,v^2> u^2 \\
%     &= \frac{2}{(1+<u^1,u^2>^2)} \sigma_1 \frac{2}{(1+<v^1,v^2>^2)} u^1 \\ &+ \frac{2}{(1+<u^1,u^2>^2)} \sigma_2 \frac{2}{(1+<v^1,v^2>^2)} < v^1, v^2> u^2
% \end{align*} % 



% \begin{equation}
%     \sum_{i=1}^\ntasks   \sum_{j=1}^{k} \sigma_j^{i} u_j^{i} v_j^{iT}.
% \end{equation}

% \begin{equation}
%     \sum_{i=1}^\ntasks   \sum_{j=1}^{k} \sigma_j^{i} \frac{u_j^{i}}{(w_U)_j} \frac{v_j^{iT}}{(w_V)_j}.
% \end{equation}


% Fixed $j$ and $i$. 

% \begin{equation}
%   \tilde{u}_j^{i} \tilde{u}_p^{l} \text{ piccolo } \forall l \in [\ntasks] \text{ and } \forall p \in k
% \end{equation}




% \begin{equation}
%   \tilde{v}_j^{i} \tilde{v}_k^{l} \text{ piccolo }
% \end{equation}

% !!!!!!!!!!!!!!!!!!!!!!!!!!!!!!!!!!!!!!!!!!!

%\section{Ablation study}
%\begin{table*}[h]
%  \resizebox{1\textwidth}{!}{
%    \begin{tabular}{cccc}
%      \toprule
%      \multirow{2}{*}{\textbf{Method}}        & \multicolumn{3}{c}{\textbf{ViT-B-32}} \\ 
%                                              \cmidrule{2-4}
%                                              & 8 tasks   & 14 tasks  & 20 task   \\ 
%                                              \midrule
%      \multicolumn{1}{c|}{Constant W}         & $63.84_{(68.87)}$ & $49.31_{(54.34)}$ & $18.44_{(20.54)}$ \\
%      \multicolumn{1}{c|}{Scaling}            & $69.26_{(74.55)}$ & $64.59_{(71.29)}$ & $60.57_{(67.36)}$ \\
%      \multicolumn{1}{c|}{Random}             & $69.94_{(75.50)}$ & $63.95_{(70.64)}$ & $60.39_{(66.83)}$ \\
%      \multicolumn{1}{c|}{Random + Scaling}   & $64.57_{(69.94)}$ & $63.87_{(70.48)}$ & $60.02_{(66.44)}$ \\
%      \rowcolor{gray!15}
%      \multicolumn{1}{c|}{\textbf{\approach}} & $80.05_{(86.17)}$ & $74.91_{(82.37)}$ & $70.66_{(77.52)}$ \\
%      \bottomrule
%    \end{tabular}
%  }
%  \caption{Ablation study showing the effect of various scaling factors}
%  \label{tab:ablation}
%\end{table*}
